# Supplementary material for: Temperature-induced increase of spin spiral periods
Source: arXiv:1703.10849 source file (2017-03-31)
Supplement: Supplementary file 1 [file supplement.pdf]

# Supplemental Material
# Temperature-induced increase of spin spiral periods

Aurore Finco[1], Levente Rózsa[1,2], Pin-Jui Hsu[1], André Kubetzka[1], Elena Vedmedenko[1], Kirsten von Bergmann[1], and Roland Wiesendanger[1]

[1]Department of Physics, University of Hamburg, D-20355 Hamburg, Germany
[2]Institute for Solid State Physics and Optics, Wigner Research Centre for Physics, Hungarian Academy of Sciences, P.O. Box 49, H-1525 Budapest, Hungary

## Experimental methods

The measurements were performed either in a low-temperature STM setup equipped with a He bath cryostat which was operated at the base temperature 8 K or at room temperature, or in a variable-temperature setup with a He-flow cryostat allowing to stabilize any sample temperature between 30 and 300 K.

Both the sample preparation and the STM measurements were realized in an ultrahigh vacuum system with a base pressure below $10^{-10}$ mbar. Different chambers were used for substrate cleaning, Fe deposition, and STM measurements. The Ir single-crystal substrate was prepared by cycles of Ar-ion sputtering at 800 eV and annealing up to 1300 °C for 60 s. The Fe film was then evaporated onto the clean substrate at elevated temperature (about 200 °C) at a deposition rate around 0.2 atomic layers per minute.

Because of contamination of the sample surface by particles desorbing from the STM body when warming up, a new sample was prepared for each increasing temperature step.

## Choice of the spin-polarized STM tip

A ferromagnetic Fe coated W tip was used at intermediate temperatures (40 to 250 K). However, at elevated temperature, the spirals appear to be affected by the stray field created by the ferromagnetic STM tip. The used Fe coating is very thick (50 to 60 layers) in order to easily obtain a stable tip magnetization, but this also induces a large stray field. Already at 43 K, as shown on Fig. 1(c) in the main text, some tip-induced fluctuations are visible. When the temperature is further increased, the effect is more pronounced and the magnetic contrast becomes weaker on some regions. These contrast differences cannot be explained by the orientation of the magnetization of the tip apex during the measurement, because the contrast is stronger in other areas with the same propagation direction. Consequently, we were not successful in imaging the spin spirals at room temperature with the ferromagnetic tip, the measurement shown in Figs. 1(f),(g) was performed with an antiferromagnetic Cr bulk tip which does not affect the magnetic structure of the sample.

## Data analysis

The periods of the spin spirals were measured using 2D Fourier transformation on the differential conductance maps, except for the room temperature data. At 300 K, line profiles were fitted to sine functions, because the resolution of the Fourier transform is not satisfactory regarding the small number of magnetic periods visible. Furthermore, only line profiles along the fast scan direction were considered because of the large thermal drift. The calibration of the STM is different for every temperature because of the strong temperature dependence of the piezoelectric coefficients in the ceramic used to build the scanner. For this reason, the images were rescaled using the height of the Ir steps as a reference, the thermal expansion of Ir between 8 K and 300 K being negligible [1].

## Mean-field calculations

As a generalization of Eq. (1) in the main text, we will consider the classical model Hamiltonian

$$H = \frac{1}{2}\sum_{p,q,i,j} J_{pq,ij}\boldsymbol{S}_{p,i}\boldsymbol{S}_{q,j} + \frac{1}{2}\sum_{p,q,i,j} \boldsymbol{D}_{pq,ij}\left(\boldsymbol{S}_{p,i}\times\boldsymbol{S}_{q,j}\right), \tag{S.1}$$

which is not restricted to nearest-neighbor interactions. We will neglect the magnetocrystalline anisotropy term, which simplifies the calculations to harmonic spin spirals. The experimental data suggest that the shape of spin spirals is close to the perfect sinusoid [2], indicating that the anisotropy plays a minor role in the system.

In the mean-field approximation, we suppose that at every lattice point, the spins have a well-defined expectation value $\left\langle\boldsymbol{S}_{p,i}\right\rangle$. Furthermore, one has to perform the replacement

$$\boldsymbol{S}_{p,i} = \left\langle\boldsymbol{S}_{p,i}\right\rangle + \left(\boldsymbol{S}_{p,i} - \left\langle\boldsymbol{S}_{p,i}\right\rangle\right) \tag{S.2}$$

in Eq. (S.1), and drop all the terms that are quadratic in the deviation from the expectation value of the spins. This leads to

$$H_{\mathrm{MF}} = -\frac{1}{2}\sum_{p,q,i,j} J_{pq,ij}\left\langle\boldsymbol{S}_{p,i}\right\rangle\left\langle\boldsymbol{S}_{q,j}\right\rangle - \frac{1}{2}\sum_{p,q,i,j}\boldsymbol{D}_{pq,ij}\left(\left\langle\boldsymbol{S}_{p,i}\right\rangle\times\left\langle\boldsymbol{S}_{q,j}\right\rangle\right) + \sum_{p,q,i,j} J_{pq,ij}\boldsymbol{S}_{p,i}\left\langle\boldsymbol{S}_{q,j}\right\rangle + \sum_{p,q,i,j}\boldsymbol{S}_{p,i}\left(\left\langle\boldsymbol{S}_{q,j}\right\rangle\times\boldsymbol{D}_{pq,ij}\right). \tag{S.3}$$

From the last two terms in Eq. (S.3), the mean field acting on the spin $\boldsymbol{S}_i$ is defined as

$$\boldsymbol{B}_{p,i} = -\sum_{q,j} J_{pq,ij}\left\langle\boldsymbol{S}_{q,j}\right\rangle - \sum_{q,j}\left\langle\boldsymbol{S}_{q,j}\right\rangle\times\boldsymbol{D}_{pq,ij}, \tag{S.4}$$

in energy dimensions.

The free energy of the system described by the noninteracting Hamiltonian, Eq. (S.3), can be expressed analytically as

$$F_{\mathrm{MF}} = -\frac{1}{2}\sum_{p,q,i,j} J_{pq,ij}\left\langle\boldsymbol{S}_{p,i}\right\rangle\left\langle\boldsymbol{S}_{q,j}\right\rangle - \frac{1}{2}\sum_{p,q,i,j}\boldsymbol{D}_{pq,ij}\left(\left\langle\boldsymbol{S}_{p,i}\right\rangle\times\left\langle\boldsymbol{S}_{q,j}\right\rangle\right) - k_{\mathrm{B}}T\sum_{p,i}\ln\left(4\pi\sinh\left(\frac{B_{p,i}}{k_{\mathrm{B}}T}\right)\frac{k_{\mathrm{B}}T}{B_{p,i}}\right). \tag{S.5}$$

The parameters $\left\langle\boldsymbol{S}_{p,i}\right\rangle$ in Eq. (S.5) must be determined in such a way as to minimize the mean-field free energy. Differentiating Eq. (S.5) with respect to the expectation values leads to the self-consistency equations

$$\left\langle\boldsymbol{S}_{p,i}\right\rangle = \left(\coth\left(\frac{B_{p,i}}{k_{\mathrm{B}}T}\right) - \frac{k_{\mathrm{B}}T}{B_{p,i}}\right)\frac{\boldsymbol{B}_{p,i}}{B_{p,i}} = \int\boldsymbol{S}_{p,i}\mathrm{e}^{\frac{\boldsymbol{B}_{p,i}\boldsymbol{S}_{p,i}}{k_{\mathrm{B}}T}}\mathrm{d}\boldsymbol{S}_{p,i}\left(\int\mathrm{e}^{\frac{\boldsymbol{B}_{p,i}\boldsymbol{S}_{p,i}}{k_{\mathrm{B}}T}}\mathrm{d}\boldsymbol{S}_{p,i}\right)^{-1}. \tag{S.6}$$

However, Eq. (S.6) has many different solutions, corresponding to stationary points in the many-dimensional free energy surface. The paramagnetic solution $\left\langle\boldsymbol{S}_{p,i}\right\rangle\equiv\boldsymbol{0}$ exists at arbitrary temperature, and the free energy of one of the ordered states must be lower than this below the critical temperature.

From the experiments it is known that the system orders into a cycloidal spin spiral state. In the mean-field model this has the form

$$\left\langle\boldsymbol{S}_{p,i}\right\rangle = \begin{bmatrix}\sin\left(kx_{p,i}\right)\\ 0\\ \cos\left(kx_{p,i}\right)\end{bmatrix}\left\langle S_p\left(k\right)\right\rangle, \tag{S.7}$$

if we assume that the wave vector $k$ is the same in all layers and points along the $x$ direction. However, the magnitude of the magnetization or order parameter $\left\langle S_p\left(k\right)\right\rangle$ may differ between the layers.

It can be proven by substitution that solutions of the form Eq. (S.7) satisfy the self-consistency equations Eq. (S.6) for arbitrary $k$ values. We introduce the simpler notations

$$B_p(k) = -\left[\sum_{q,j} J_{pq,ij} \cos\left(k\left(x_{p,i} - x_{q,j}\right)\right)\left\langle S_q(k)\right\rangle + D_{pq,ij} \sin\left(k\left(x_{p,i} - x_{q,j}\right)\right)\left\langle S_q(k)\right\rangle\right] \tag{S.8}$$

and

$$\mathcal{J}_{pq}(k) = \sum_{q,j} J_{pq,ij} \cos\left(k\left(x_{p,i} - x_{q,j}\right)\right) + D_{pq,ij} \sin\left(k\left(x_{p,i} - x_{q,j}\right)\right), \tag{S.9}$$

with $D_{pq,ij}$ being the in-plane component of the Dzyaloshinsky–Moriya vector perpendicular to the $x$ direction. Equations (S.8)-(S.9) do not depend on the lattice site $i$ due to the translational invariance of the Heisenberg and Dzyaloshinsky–Moriya exchange interactions. The free energy Eq. (S.5) may be expressed as

$$\frac{1}{N}F_{\mathrm{MF}}(k) = -\frac{1}{2}\sum_{p,q}\mathcal{J}_{pq}(k)\left\langle S_p(k)\right\rangle\left\langle S_q(k)\right\rangle - \sum_{p} k_{\mathrm{B}}T \ln\left(4\pi \sinh\left(\frac{B_p(k)}{k_{\mathrm{B}}T}\right)\frac{k_{\mathrm{B}}T}{B_p(k)}\right), \tag{S.10}$$

where $N$ is the number of spins in a single layer. Equations (2)-(4) in the main text are specific forms of Eqs. (S.8)-(S.10), including only nearest-neighbor interactions. The free energy minimum is obtained by optimizing Eq. (S.10) with respect to $k$.

As mentioned in the main text, the temperature dependence of the order parameter is different between the layers, which induces the change in the spin spiral wave vector with temperature. This is illustrated in Fig. S1, with the parameters used in the main text. The different behavior of the order parameters is connected to the different strength of the coupling constants in the different layers. This strength may be characterized by the mean-field critical temperature,

$$k_{\mathrm{B}}T_{p,\mathrm{c}} = -\frac{\mathcal{J}_{pp}\left(k_p\right)}{3}, \tag{S.11}$$

where the minimization with respect to $k$ must be performed for each layer separately, yielding the $k_p$ values. For the parameters summarized in Fig. 2(d), rescaled by a factor of 0.71 as mentioned in the main text, one obtains $\frac{2\pi}{k_1} = 1\,\mathrm{nm}$, $T_{1,\mathrm{c}} = 77\,\mathrm{K}$; $\frac{2\pi}{k_2} = 3\,\mathrm{nm}$, $T_{2,\mathrm{c}} = 109\,\mathrm{K}$; and $\frac{2\pi}{k_3} = 473\,\mathrm{nm}$, $T_{3,\mathrm{c}} = 348\,\mathrm{K}$. Figure S1 also demonstrates that the whole system only has a single critical temperature due to the presence of the interlayer couplings.

The parameter set used during the calculations in the main text (see Fig. 2(d)) is not unique, we found that it was possible to reasonably reproduce the experimental data with several different choices of the coupling coefficients. This is partly due to the strain effect observed in the experiments, inducing a significant variance in the observed periods at a single temperature. The critical temperature of the system is also a variable parameter, since the experiments only confirmed that this must be above room temperature for the triple layer. Finally, it is known that competing ferromagnetic and antiferromagnetic exchange interactions may also influence the period of the spin spiral ordering [3], and the importance of this frustration has been demonstrated recently for ultrathin film systems [4–7] similar to the Fe on Ir(111) discussed in this paper. We checked that the temperature dependence may also be reproduced by considering frustrated exchange interactions, which makes it unnecessary to suppose $D_{11} > |J_{11}|$ used in the main text, which is unlikely to occur when the interaction coefficients are determined from *ab initio* methods.

However, the coupling constants used in the main text provide a simple picture of what is necessary for obtaining such a significant increase of the spin spiral period with temperature. One important point is the intralayer couplings defining different periods and mean-field critical temperatures in the atomic layers as discussed above. For the interlayer couplings the calculations indicated that we must choose $|J_{12}| > |J_{23}|$, which is necessary to explain why the period increases faster at higher temperature, by approximately the same factor between 4 K and 250 K as between 250 K and room temperature.

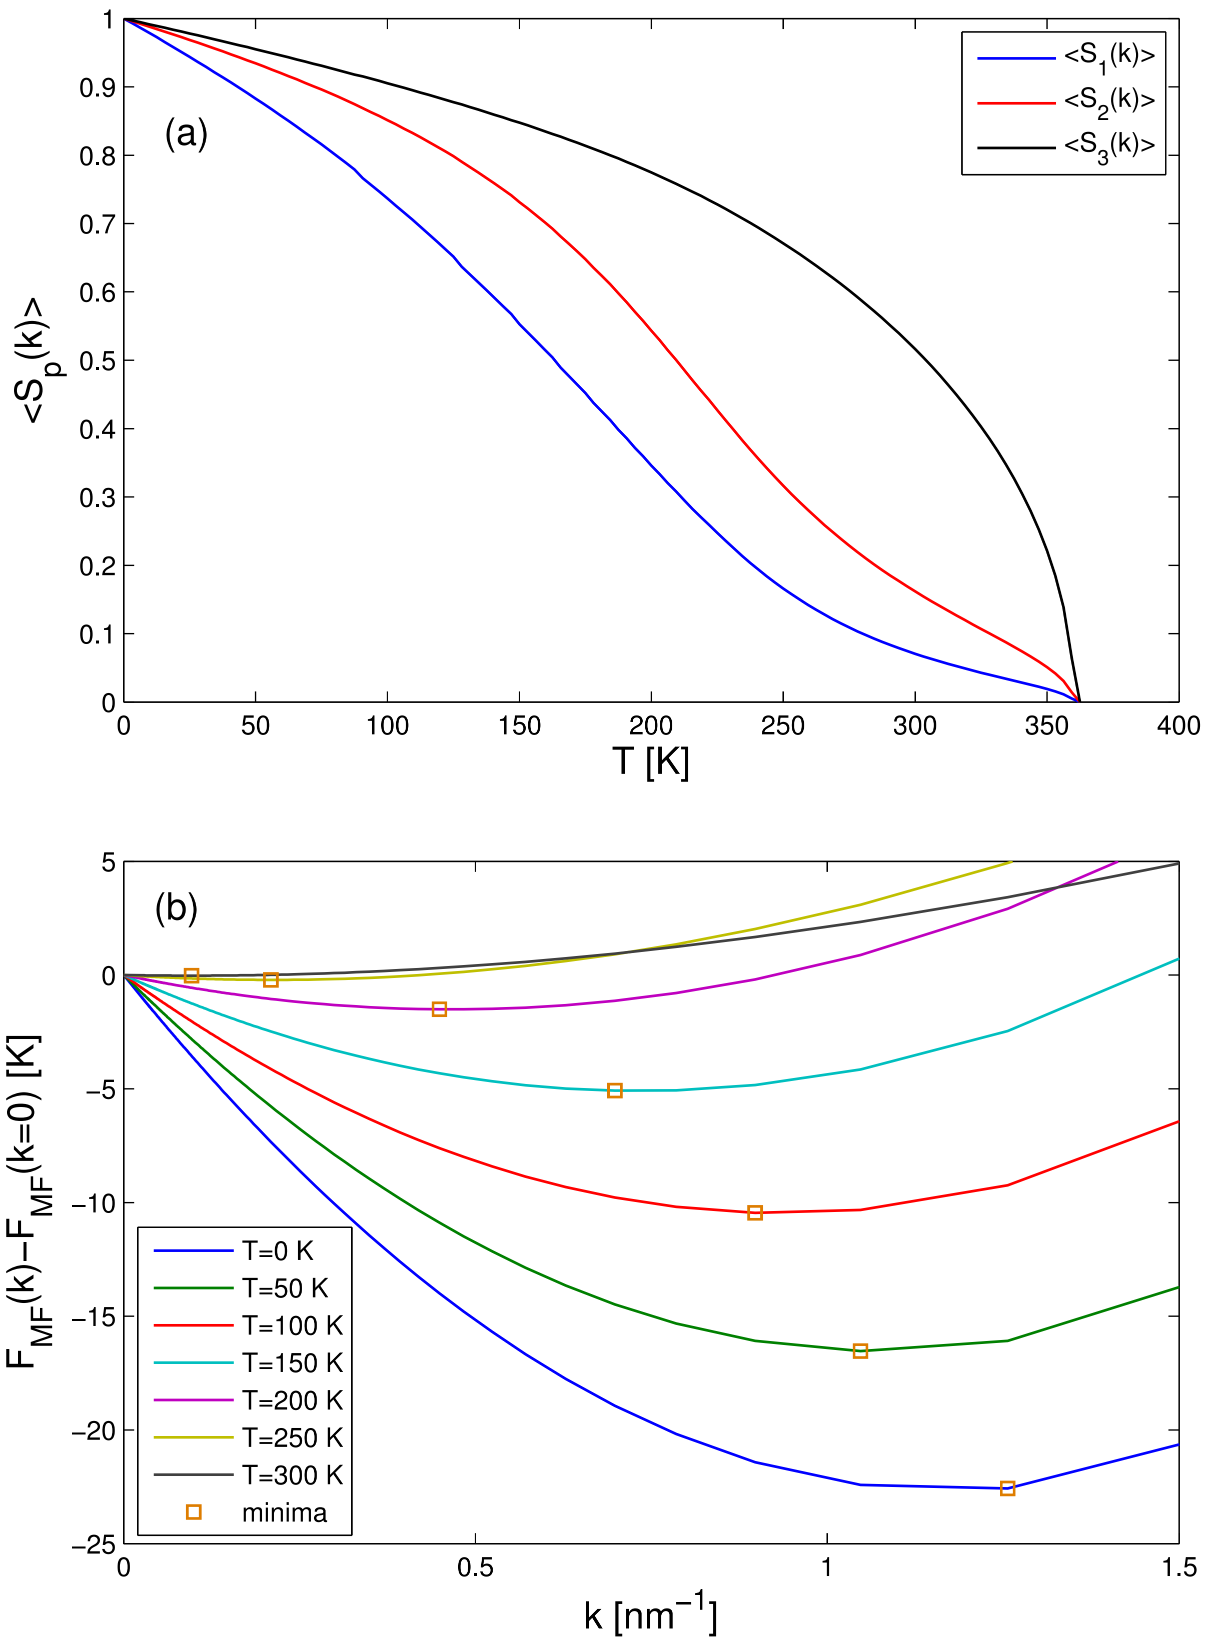


Figure S1: (a) Order parameters $\langle S_p(k) \rangle$ as a function of temperature in the different layers in the mean-field approximation. At each temperature, the wave vector is chosen to minimize the total free energy. (b) Free energy per spin $F_{\mathrm{MF}}$ in the mean-field approximation as a function of the wave vector $k$, for selected temperature values $T$. The coupling constants from Fig. 2(d) in the main text were used, all of them rescaled by a factor of 0.71 to obtain a better agreement with the experimental data for the temperature range.

## Monte Carlo simulations

Although the mean-field model already predicts the increase of the spin spiral period with temperature, we also performed Monte Carlo simulations using the model Hamiltonian Eq. (1) in the main text, which were expected to improve upon the model calculations in several aspects. As already discussed above, the mean-field calculation significantly overestimates the critical temperature, which was handled by a rescaling of the coupling constants or equivalently the temperature range. Even after the rescaling, it can be seen in Fig. 2(a) in the main text that the Monte Carlo simulations predict a larger curvature around 250 K for the period-temperature data than the mean-field model, and this actually gives better agreement with the experiments. This can be attributed to the role of spin fluctuations, which are neglected in the mean-field model. However, the most important objective of the Monte Carlo simulations is confirming that the interlayer couplings are sufficiently strong to force all three layers into a spin spiral state with the same period at every temperature. Although this was a crucial assumption in the mean-field model, it is only possible to give weak approximations about its validity without the simulations.

The program swept over the lattice at every Monte Carlo step, and updated the orientations of the spins following single-spin Metropolis dynamics. From the spin configurations, we determined the Fourier transforms in each layer,

$$\boldsymbol{S}_{p,\boldsymbol{k}} = \frac{1}{N}\sum_{i} \mathrm{e}^{-\mathrm{i}\boldsymbol{k}\boldsymbol{R}_{p,i}}\boldsymbol{S}_{p,i}, \tag{S.12}$$

then calculated the static structure factor by averaging,

$$S_p(\boldsymbol{k}) = \sum_{\alpha=x,y,z}\left\langle\left|S^{\alpha}_{p,\boldsymbol{k}}\right|^2\right\rangle. \tag{S.13}$$

Finding the maximum of $S_p(\boldsymbol{k})$ with respect to the wave vector yields the period of the spin spiral, or of other types of noncollinear order in the system [8]. In the current case, it also enabled us to check that the spin order remained the same in all three layers at all temperatures, which we also confirmed by looking at selected spin configurations in real space.

The Monte Carlo simulations shown in Fig. 2(a) were performed for three layers of atoms in perfect fcc stacking with the two-dimensional lattice constant of the Ir(111) surface, $a = 0.271$ nm. We used a lattice size of $256a \times 16\sqrt{3}a \approx 70 \times 7.5$ nm (24576 spins) for temperatures up to 250 K and $1024a \times 16\sqrt{3}a \approx 280 \times 7.5$ nm (98304 spins) between 250 K and room temperature. Although the larger lattice size increased the simulation time significantly, it was necessary for improving the resolution of Fourier transformation in order to determine the period more accurately at higher values. The wave vector of the spin spiral was parallel to the long edge of the simulation sample at all temperatures. Free boundary conditions were considered along the short edges of the sample, which made it easier for the system to achieve the equilibrium wave vector at each temperature during thermalization, and periodic boundary conditions were used along the long edges. The elongated simulation cell emulated the dislocation lines guiding the spin spirals in the experiments. Since in the model calculations the interactions were isotropic (in the sense that they took the same values for all neighbors), the elongated simulation cell also served the purpose of excluding spin configurations with wave vectors uniformly distributed along a circle [8], which would be expected from the model but would contradict experimental findings. At every temperature, the system was thermalized for $2 \times 10^5$ steps, then the averaging was performed over $10^6$ steps.

## References


[1] J. W. Arblaster. Crystallographic Properties of Iridium. *Plat. Met. Rev.* 54.2 (2010), pp. 93–102.

[2] A. Finco, P.-J. Hsu, A. Kubetzka, K. von Bergmann, and R. Wiesendanger. Tailoring noncollinear magnetism by misfit dislocation lines. *Phys. Rev. B* 94.21 (2016), p. 214402.

[3] Y. A. Izyumov. Modulated, or long-periodic, magnetic structures of crystals. *Sov. Phys. Usp.* 27.11 (1984), p. 845.

[4] S. Heinze, K. von Bergmann, M. Menzel, J. Brede, A. Kubetzka, R. Wiesendanger, G. Bihlmayer, and S. Blügel. Spontaneous atomic-scale magnetic skyrmion lattice in two dimensions. *Nat. Phys.* 7.9 (2011), pp. 713–718.

[5] B. Dupé, M. Hoffmann, C. Paillard, and S. Heinze. Tailoring magnetic skyrmions in ultra-thin transition metal films. *Nat. Commun.* 5 (2014), p. 4030.

[6] L. Rózsa, L. Udvardi, L. Szunyogh, and I. A. Szabó. Magnetic phase diagram of an Fe monolayer on W(110) and Ta(110) surfaces based on *ab initio* calculations. *Phys. Rev. B* 91.14 (2015), p. 144424.

[7] L. Rózsa, A. Deák, E. Simon, R. Yanes, L. Udvardi, L. Szunyogh, and U. Nowak. Skyrmions with Attractive Interactions in an Ultrathin Magnetic Film. *Phys. Rev. Lett.* 117.15 (2016), p. 157205.

[8] L. Rózsa, E. Simon, K. Palotás, L. Udvardi, and L. Szunyogh. Complex magnetic phase diagram and skyrmion lifetime in an ultrathin film from atomistic simulations. *Phys. Rev. B* 93.2 (2016), p. 024417.
